# Supplementary material for: Fast View Synthesis of Casual Videos with Soup-of-Planes
Source: arXiv:2312.02135 source file (2024-07-19)
Supplement: Supplementary file 2 [file tb_supp_scene_flow.tex]

\makeatletter
\newcommand*\tablesupponesize{%
  \@setfontsize\tablesupponesize{6}{10.0}%
}
\makeatother

\begin{table*}[t]
\caption{\textbf{Ablation on scene flow regularization.}
Although the scene flow regularization $\L_{sf}$ can improve the scores of three examples by better aligning with the ground-truths, the quality of the other four examples degrades due to the over-smoothed dynamic depths caused by the regularization. Additionally, the scene flow regularization doubles the training time. Hence, we disable the scene flow regularization by default. Without the regularization, our method can still render visually plausible dynamics in spite of some slight misalignments with the ground truth. We encourage our readers to view our %\href{run:index.html}{demo webpage} 
demo webpage to see the video synthesis results of casual videos.
}
\tablesupponesize
\resizebox{\textwidth}{!}{\begin{tabular}{L{1.8cm}|c|ccccccc|c}
\hline
\multicolumn{1}{c|}{PSNR \textuparrow / LPIPS \textdownarrow} & Train time & Jumping & Skating & Truck & Umbrella & Balloon1 & Balloon2 & Playground & Average \\ \hline
Ours w/ $\L_{sf}$ & 33 min & 22.36 / 0.121 & 28.99 / 0.062 & 25.07 / 0.093 & \textbf{23.91} / \textbf{0.094} & {22.36} / {0.121} & \textbf{25.31} / \textbf{0.072} & \textbf{22.76} / \textbf{0.070} & 24.55 / {0.086} \\
Ours w/o $\L_{sf}$ & 15 min & \textbf{23.45} / \textbf{0.100} & \textbf{29.98} / \textbf{0.045} & \textbf{25.22} / \textbf{0.090} & 23.24 / {0.096} & \textbf{23.75} / \textbf{0.079} & 24.15 / 0.081 & 22.19 / {0.074} & \textbf{24.57} / \textbf{0.081} \\ 
\hline
\end{tabular}
}
\label{tbl:supp_nvidia_scene_flow}
\end{table*}
