# Supplementary material for: Fast View Synthesis of Casual Videos with Soup-of-Planes
Source: arXiv:2312.02135 source file (2024-07-19)
Supplement: Supplementary file 3 [file fig_supp_3dgs_ambiguity.tex]

\begin{wrapfigure}{r}{0.25\textwidth}
\centering
\vspace{-0.6cm}\includegraphics[trim={0.1cm 4.4cm 27cm 0.2cm},clip,keepaspectratio,scale=0.3]{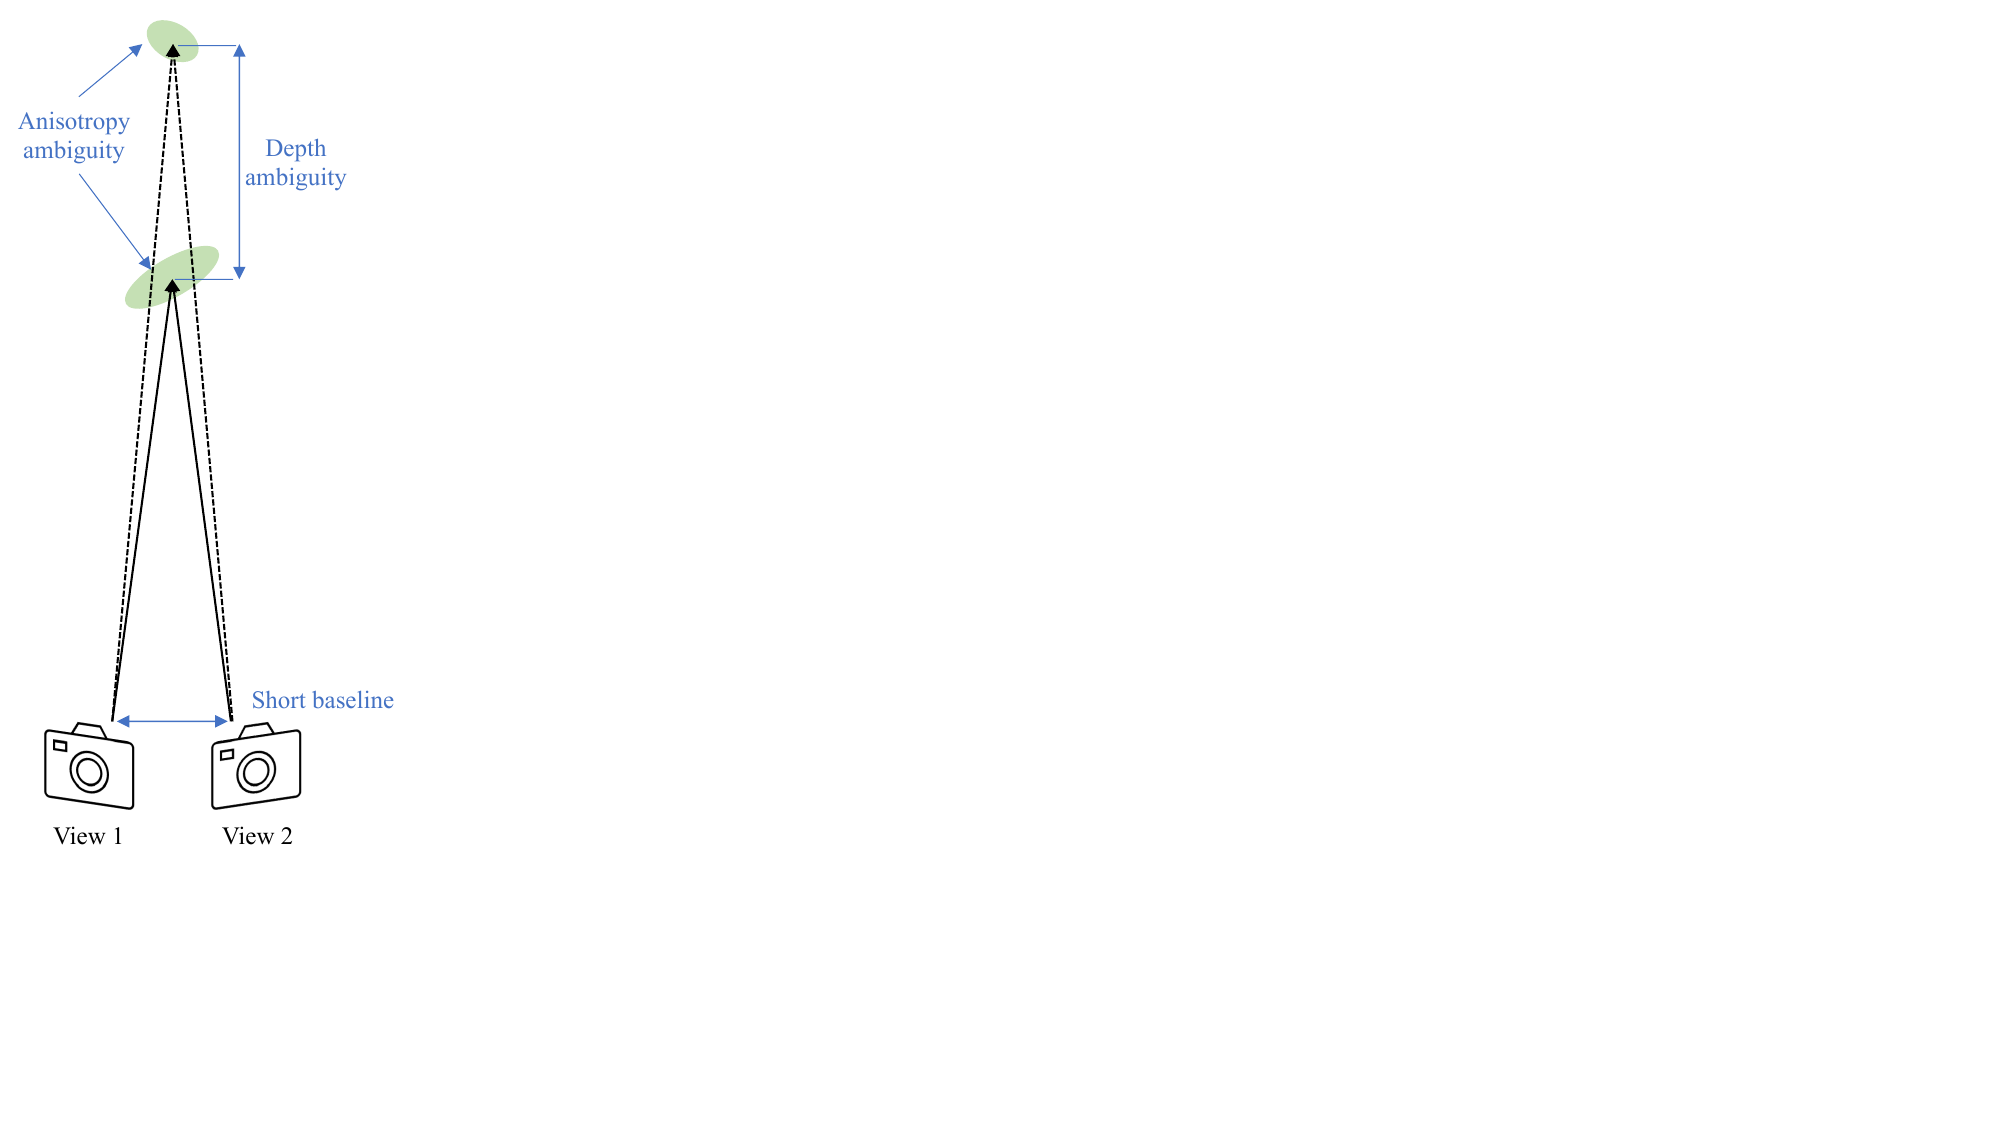}
% \vspace{-8mm}
\caption{{\textbf{Ambiguities of 3DGS in weak-parallax scenes.}}
}
\vspace{-7mm}
\label{fig:supp_plane_visualization}
\end{wrapfigure}
