# Supplementary material for: Fast View Synthesis of Casual Videos with Soup-of-Planes
Source: arXiv:2312.02135 source file (2024-07-19)
Supplement: Supplementary file 4 [file fig_supp_model_size.tex]

\begin{figure}
\includegraphics[trim={0.5cm 14cm 14cm 0.1cm},clip,width=\linewidth]{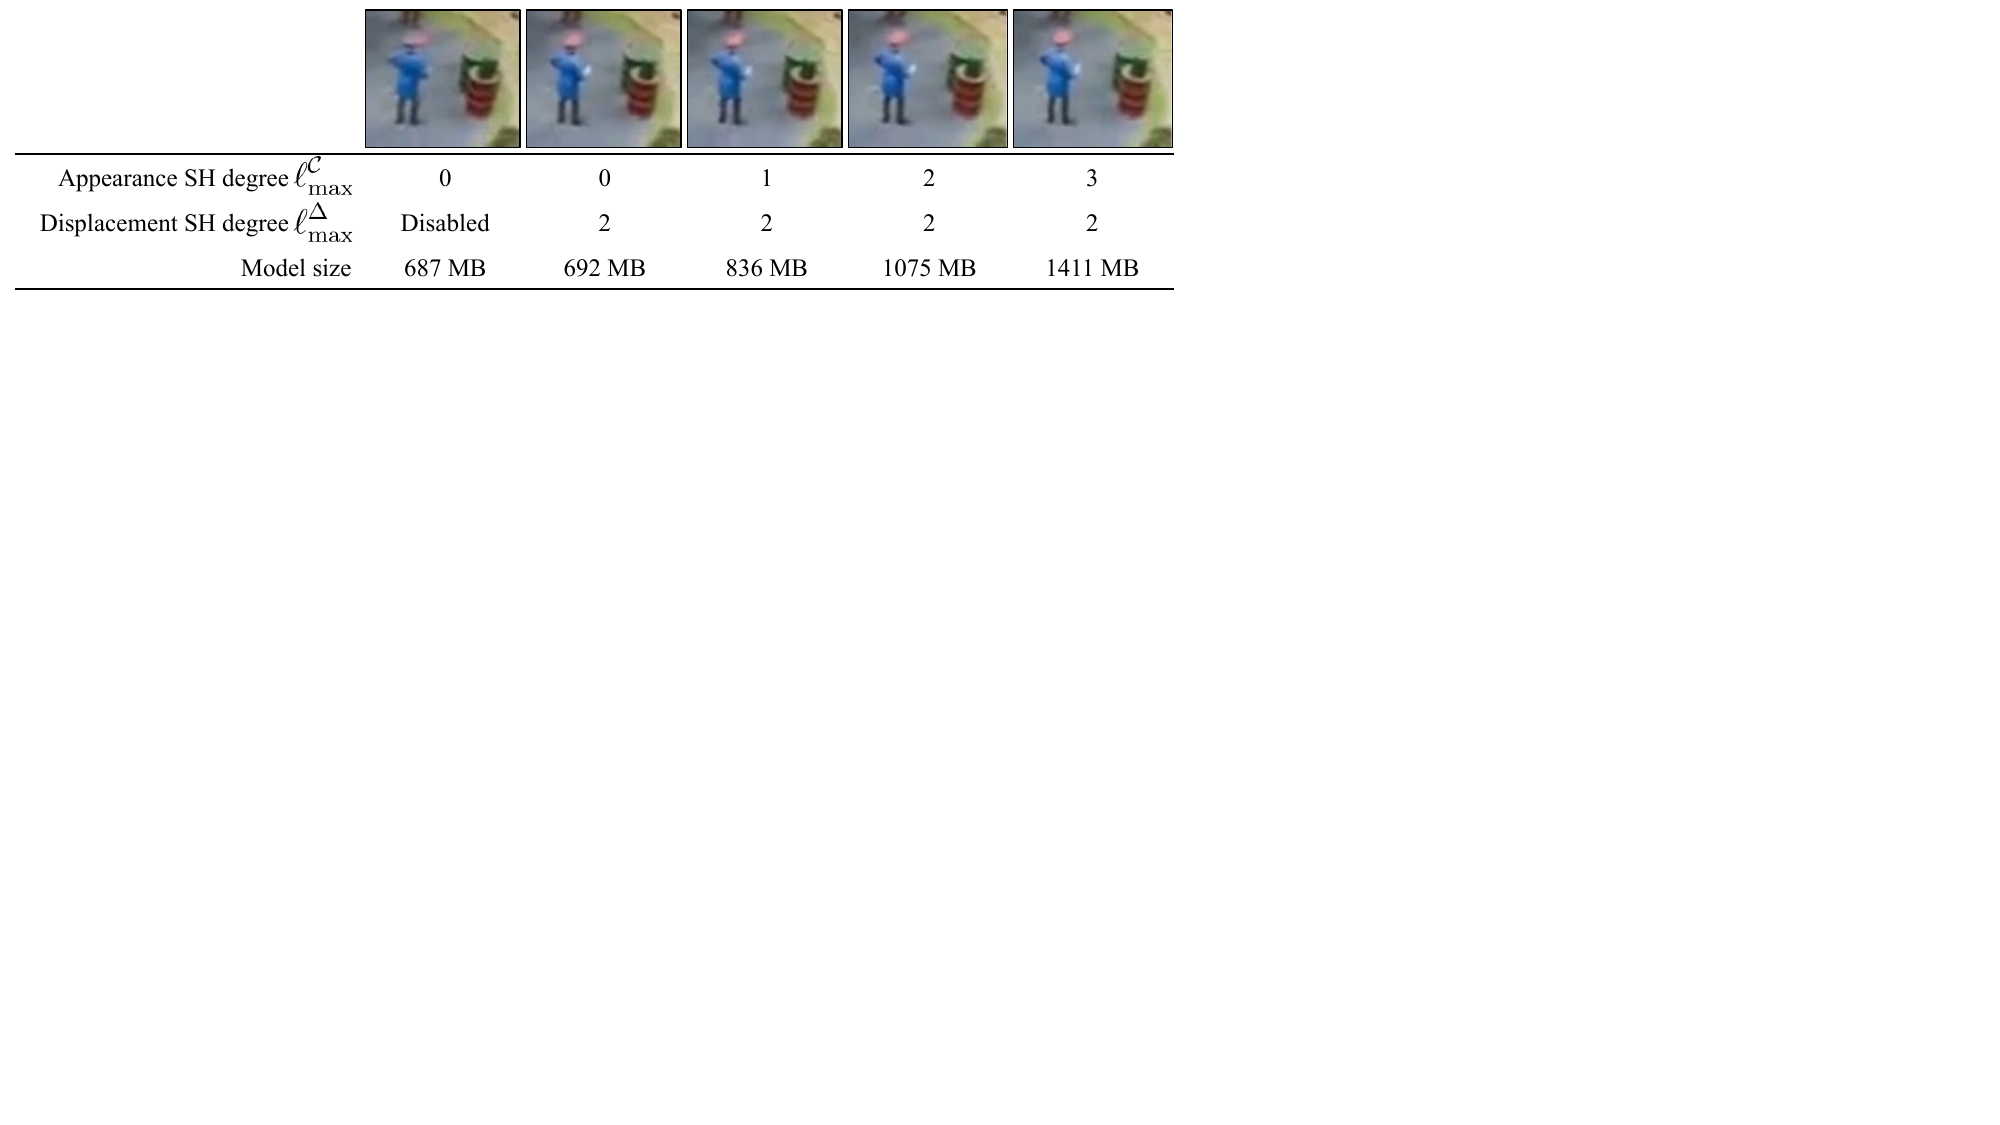}
\vspace{-4mm}
\caption{{\textbf{Model size comparison.}}
We present the trade-off between the visual quality and model size, focusing primarily on the view-dependent appearance texture maps $\C^{0..\ell_{\max}^{\C}}$.
However, it's important to note that in the first and second columns, our proposed view-dependent displacement maps $\Delta^{0..\ell_{\max}^{\Delta}}$ are capable of retaining more complex scene details even without relying on view-dependent appearance, and this comes at a mere additional 5MB in size.
}
\vspace{-7mm}
\label{fig:supp_model_size}
\end{figure}
