# Supplementary material for: Fast View Synthesis of Casual Videos with Soup-of-Planes
Source: arXiv:2312.02135 source file (2024-07-19)
Supplement: Supplementary file 5 [file fig_supp_nvidia_part2.tex]

\begin{figure*}[ht]
    \centering
    \frame{\includegraphics[width=0.24\linewidth]{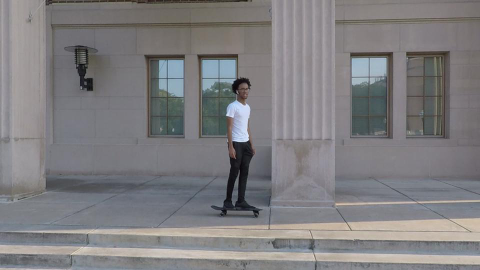}}
    \frame{\includegraphics[width=0.24\linewidth]{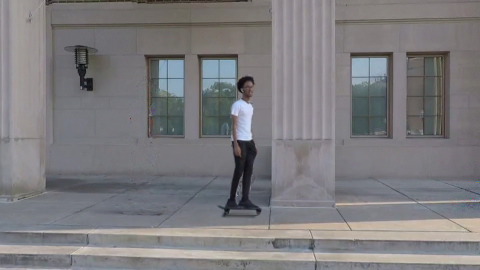}}
    \frame{\includegraphics[width=0.24\linewidth]{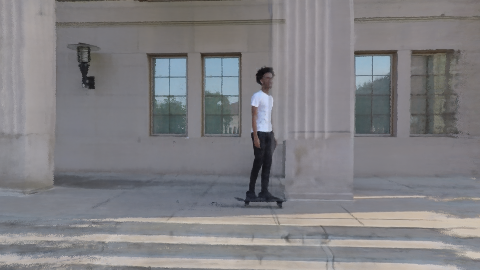}}
    \frame{\includegraphics[width=0.24\linewidth]{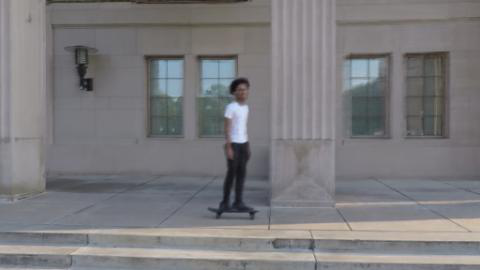}}
    \\
    \vspace{-1mm}
    \begin{subfigure}{0.24\linewidth}\centering\small
        Ground Truth
    \end{subfigure}
    \begin{subfigure}{0.24\linewidth}\centering\small
        Ours
    \end{subfigure}
    \begin{subfigure}{0.24\linewidth}\centering\small
        HyperNeRF~\cite{gao2021dynerf}
    \end{subfigure}
    \begin{subfigure}{0.24\linewidth}\centering\small
        NSFF~\cite{nsff}
    \end{subfigure}
    \\
    \vspace{1.5mm}
    \frame{\includegraphics[width=0.24\linewidth]{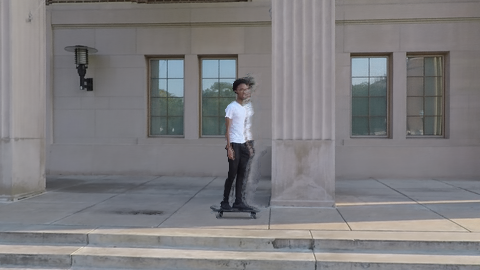}}
    \frame{\includegraphics[width=0.24\linewidth]{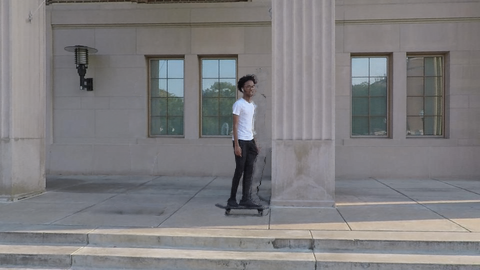}}
    \frame{\includegraphics[width=0.24\linewidth]{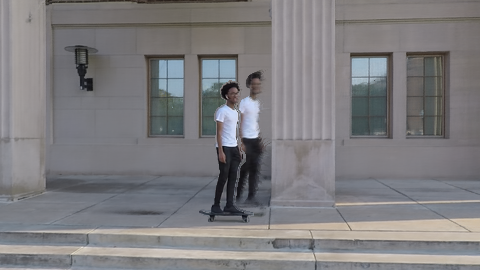}}
    \frame{\includegraphics[width=0.24\linewidth]{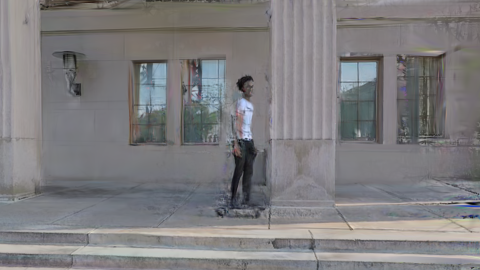}}
    \\
    \vspace{-1mm}
    \begin{subfigure}{0.24\linewidth}\centering\small
        DynNeRF~\cite{gao2021dynerf}
    \end{subfigure}
    \begin{subfigure}{0.24\linewidth}\centering\small
        RoDynRF~\cite{robustdynrf}
    \end{subfigure}
    \begin{subfigure}{0.24\linewidth}\centering\small
        MonoNeRF~\cite{tian2023mononerf}
    \end{subfigure}
    \begin{subfigure}{0.24\linewidth}\centering\small
        4D-GS~\cite{wu4dgaussians}
    \end{subfigure}
    \\
    %%%%%%%%%%%%%%%%%%%%%%%%%%%%%%%%%%%%%%%%%%%%%%%%
    \vspace{4mm}
    \frame{\includegraphics[width=0.24\linewidth]{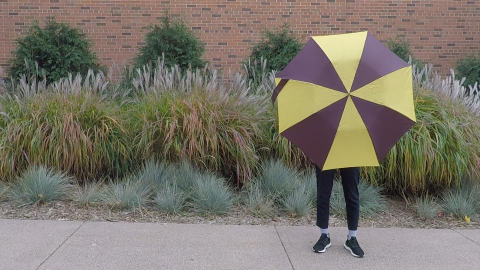}}
    \frame{\includegraphics[width=0.24\linewidth]{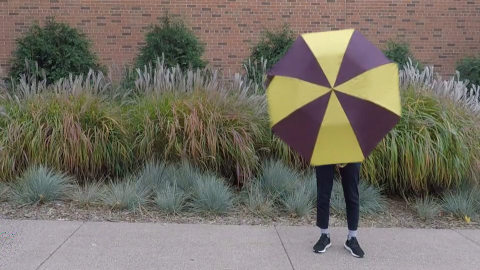}}
    \frame{\includegraphics[width=0.24\linewidth]{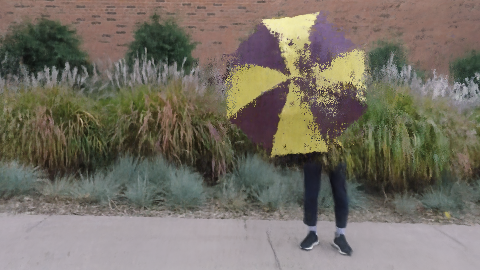}}
    \frame{\includegraphics[width=0.24\linewidth]{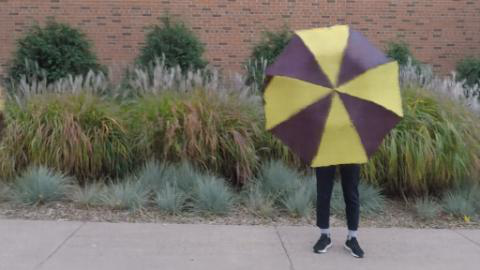}}
    \\
    \vspace{-1mm}
    \begin{subfigure}{0.24\linewidth}\centering\small
        Ground Truth
    \end{subfigure}
    \begin{subfigure}{0.24\linewidth}\centering\small
        Ours
    \end{subfigure}
    \begin{subfigure}{0.24\linewidth}\centering\small
        HyperNeRF~\cite{gao2021dynerf}
    \end{subfigure}
    \begin{subfigure}{0.24\linewidth}\centering\small
        NSFF~\cite{nsff}
    \end{subfigure}
    \\
    \vspace{1.5mm}
    \frame{\includegraphics[width=0.24\linewidth]{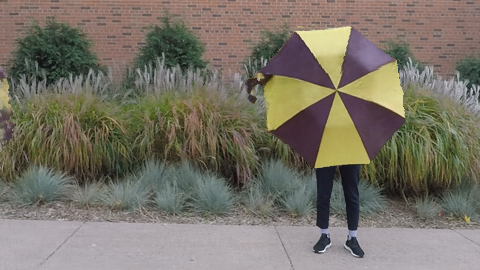}}
    \frame{\includegraphics[width=0.24\linewidth]{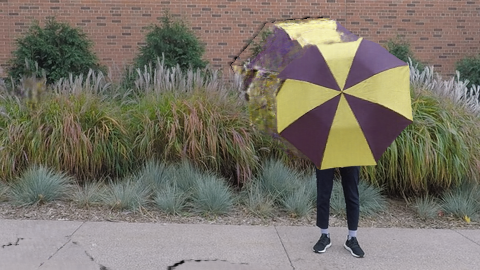}}
    \frame{\includegraphics[width=0.24\linewidth]{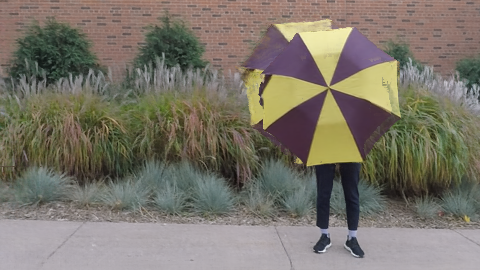}}
    \frame{\includegraphics[width=0.24\linewidth]{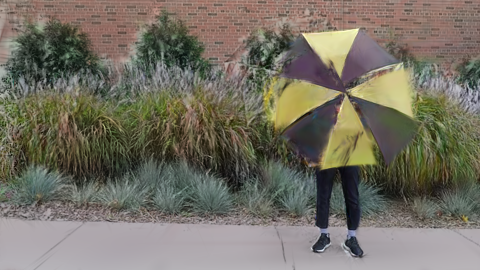}}
    \\
    \vspace{-1mm}
    \begin{subfigure}{0.24\linewidth}\centering\small
        DynNeRF~\cite{gao2021dynerf}
    \end{subfigure}
    \begin{subfigure}{0.24\linewidth}\centering\small
        RoDynRF~\cite{robustdynrf}
    \end{subfigure}
    \begin{subfigure}{0.24\linewidth}\centering\small
        MonoNeRF~\cite{tian2023mononerf}
    \end{subfigure}
    \begin{subfigure}{0.24\linewidth}\centering\small
        4D-GS~\cite{wu4dgaussians}
    \end{subfigure}
    \\
    
\vspace{-3mm}
\caption{
\textbf{Visual comparison on the NVIDIA dataset.} 
\vspace{-0.1in}
}
\label{fig:supp_nvidia_visual2}
\end{figure*}
