# Supplementary material for: Fast View Synthesis of Casual Videos with Soup-of-Planes
Source: arXiv:2312.02135 source file (2024-07-19)
Supplement: Supplementary file 6 [file fig_supp_plane_visualization.tex]

\begin{figure}
\includegraphics[trim={0.155cm 14cm 10.45cm 0.94cm},clip,width=\linewidth]{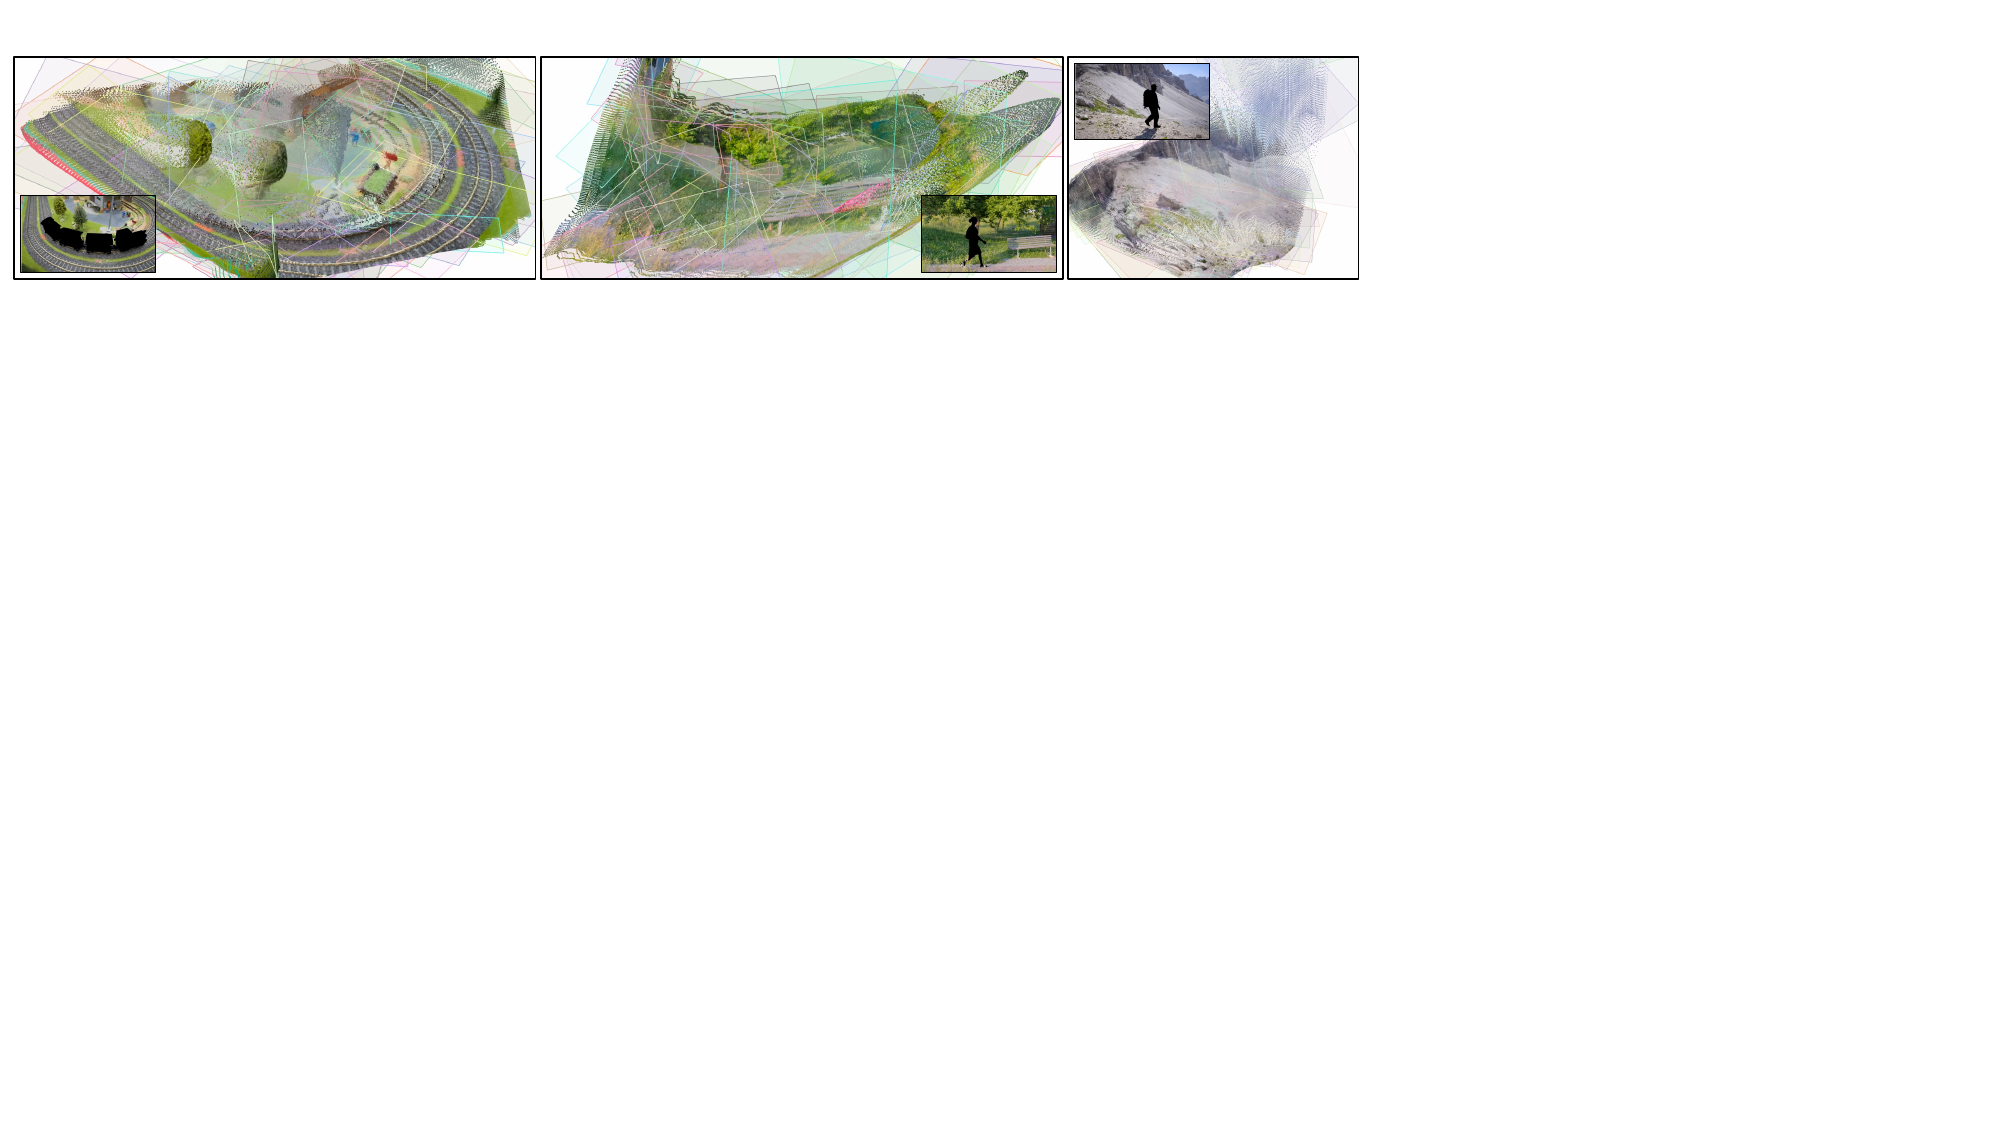}
\vspace{-8mm}
\caption{{\textbf{Visualizations of soup-of-planes.}}
We fit a set of 3D-oriented planes onto the static-scene point cloud in the plane initialization step.
}
\vspace{-7mm}
\label{fig:supp_plane_visualization}
\end{figure}
