# Supplementary material for: Fast View Synthesis of Casual Videos with Soup-of-Planes
Source: arXiv:2312.02135 source file (2024-07-19)
Supplement: Supplementary file 7 [file fig_supp_view_dependent_displacement.tex]

\begin{figure}
\centering
\includegraphics[trim={0.1cm 11cm 19cm 0.1cm},clip,width=0.7\linewidth]{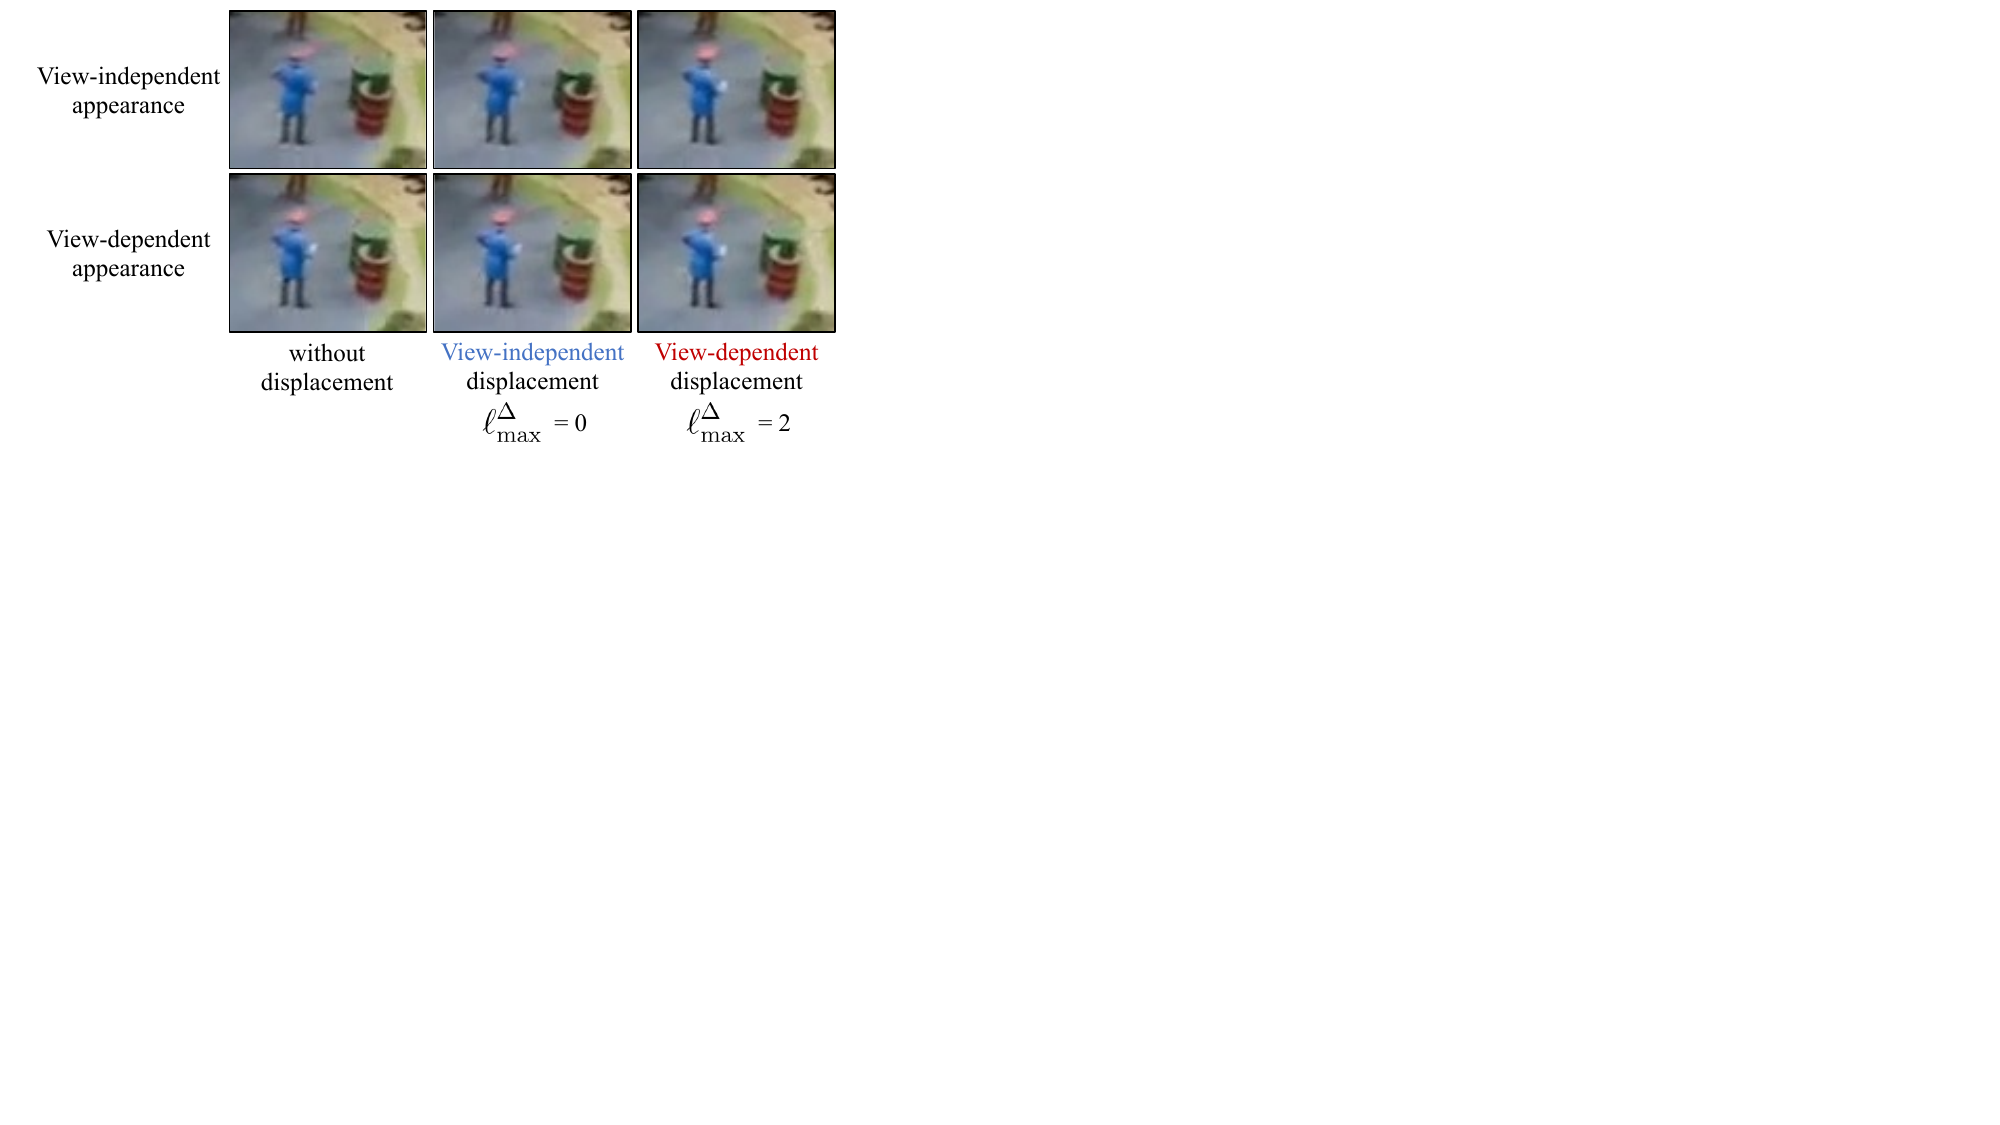}
\vspace{-4mm}
\caption{{\textbf{Efficacy of view-dependent texture displacement.}}
We compare the proposed view-dependent texture displacement with two baseline approaches. In the middle column, we employ a view-independent displacement by setting $\ell_{\max}^{\Delta}$ to 0. While view-independent displacement can help redistribute texture space to preserve high-frequency details more effectively than without texture displacement (left column), it remains inadequate in accurately modeling the diverse ray-plane intersections of a complex surface. In contrast, the proposed view-dependent texture displacement handles the complex geometry, resulting in superior rendering quality (right column).
}
% \vspace{-7mm}
\label{fig:supp_view_dependent_displace}
\end{figure}
