# Supplementary material for: Fast View Synthesis of Casual Videos with Soup-of-Planes
Source: arXiv:2312.02135 source file (2024-07-19)
Supplement: Supplementary file 8 [file supp_tb_render_time.tex]

\begin{table}
\caption{\textbf{Rendering runtime breakdown.} The experiment is conducted on a single A100 GPU with an 80-frame input video of 860\texttimes 480 resolution. The proposed method achieves real-time rendering at 27 FPS.}
\scriptsize
\centering
\begin{tabular}{lL{3.8cm}r}
\hline
\multicolumn{2}{l}{Rendering step} & \multicolumn{1}{c}{Runtime (ms)} \\ \hline
\multirow{4}{*}{Static} & Obtain view-dep. texture & 1.99 \\
 & Plane warping & 12.42 \\
 & Pixelwise depth sorting & 0.12 \\
 & Plane composition & 0.27 \\ \hline
\multirow{2}{*}{Dynamic} & Neighboring blending & 21.28 \\
 & Forward splatting & 1.35 \\ \hline
\multicolumn{2}{l}{Static-dynamic composition} & 0.09 \\ \hline
Total &  & 37.52 \\ \hline
\end{tabular}

\label{tbl:supp_rendering_runtime_breakdown}
\end{table}
