# Supplementary material for: Fast View Synthesis of Casual Videos with Soup-of-Planes
Source: arXiv:2312.02135 source file (2024-07-19)
Supplement: Supplementary file 9 [file supp_tb_train_time.tex]

\begin{table}
\caption{\textbf{Training runtime breakdown.} We run the experiment on a single A100 GPU with an 80-frame input video of 860x480 resolution. Our method is efficient to supervise and trains on casual videos within 15 minutes.}
\scriptsize
\centering
\begin{tabular}{lL{3.2cm}r}
\hline
\multicolumn{2}{l}{Training step} & \multicolumn{1}{l}{Runtime (sec)} \\ \hline
\multirow{3}{*}{Initialization} & Plane geometry fitting & 22.2 \\
 & Plane texture & 1.2 \\
 & Dynamic model & 2.4 \\ \hline
\multicolumn{2}{l}{Scene representation optimization} & 782.0 \\ \hline
\multicolumn{2}{l}{Total} & 807.8 \\ \hline
\end{tabular}

\label{tbl:supp_training_runtime_breakdown}
\end{table}
